# Supplementary material for: A snapshot review on soft-materials assembly design utilizing machine learning methods
Source: arXiv:2405.03805 source file (2024-05-06)
Supplement: Supplementary file 1 [file si_arxiv.pdf]

# Supplementary Information (SI): A snapshot review on soft-materials assembly design utilizing machine learning methods

Maya M. Martirossyan[1], Hongjin Du[1], Julia Dshemuchadse[1*], Chrisy Xiyu Du[2*]

[1]Department of Materials Science and Engineering, Cornell University, Ithaca, 14853, NY, USA.
[2]Department of Mechanical Engineering, University of Hawaiʻi at Mānoa, Honolulu, 96822, HI, USA.

*Corresponding author(s). E-mail(s): jd732@cornell.edu; xiyudu@hawaii.edu;
Contributing authors: mmm457@cornell.edu; hd329@cornell.edu;

## 1 Other descriptor types for self-assembly studies

*Thermodynamics-inspired features and methods.* While thermodynamics-inspired features are not as commonly used as those that focus primarily on structure, they are yet another way to create order metrics for studying critical phenomena and system behavior in assembling systems. Three general categories exist under this umbrella: energy-based features, entropy-based features, and ML-based diffusion models (which differ in that it is the method, rather than the features, that is derived from thermodynamics).

An example of an energy-based feature—shown to be a poor predictor of glassy dynamics—is the potential energy summed over a particle's nearest neighbors (or "inherent structure") [1]. The Bag of Bonds model [2] is an instance of using ML to fit the energies of bonds—rather than for each atom type—that relies similarly on the enthalpic interactions between particles for training. However, this paper points out that this type of feature is insensitive to geometry and sensitive only to interparticle distance (i.e., it could not distinguish two molecules with the same bonds but in different orientations).

*Entropy-inspired features and methods.* Entropy-based approaches are more commonly utilized than energy-based ones to study the behavior of an ensemble. The free volume [3] that a particle has available to move is intrinsically tied to a particle's entropy and has been employed to understand grain-coarsening mechanisms in colloidal crystals [4]. Another approach using an entropy-based "local fingerprint" [5] projects the excess entropy metric—which is based on the radial distribution function—onto individual particles. Finally, a measure of information entropy based on the change in length of a compressed string representing particle positions—called computable information density (CID) [6]—has been shown to identify phase transitions in both lattice and continuous systems. While most of these approaches have not yet been utilized in conjunction with ML, entropy-based order metrics have been machine-learned in multi-component alloys using the Kullback–Leibler divergence to identify chemical "randomness" (or a lack thereof) [7]. This approach is based on the idea of relative entropy and could be utilized in a modular fashion with other types of chosen features.

# 2 Property design for soft materials

*Mechanical properties.* Due to their direct connection with materials structure, mechanical properties are often the most readily modeled. ML-models have been devised to predict strain-stiffening in granular "molecules" (composed of sphere-union clusters) with an evolutionary algorithm [8], plasticity in amorphous materials with support vector machines (SVMs) [9–11], effective stiffness of composites with convolutional neural networks (CNNs) [12], stiffness matrix components in metamaterial microstructures with a variational autoencoder (VAE) [13], viscoelastic properties (glassy modulus, rubbery modulus, and $\tan\delta$ peak) of polymer nanocomposites with a combination of convolutional neural networks and multi-task learning [14], increased resistance to shear cracking in nanocomposites with a deep learning model using both CNN and genetic algorithm components [15], and anisotropic elastic stiffness in biomimetic, bone-like spinodoid topologies using deep neural networks [16]. Predictive models such as those have enabled, for example, the design of maximum- and minimum-stress filler morphologies in filled rubbers with CNNs [17] and the yield stress and viscosity in polymeric dispersants for facilitating the flow of particle suspensions with LASSO regression (least absolute shrinkage and selection operator, i.e., L1 regularization) [18].

*Thermodynamic or phase properties.* Thermodynamic or phase properties have also been modeled successfully with machine-learning approaches. In addition to, for example, modeling of the antifreeze activity of proteins with a neural network [19] or glass transition temperatures of polymers with random forest models or a combined kernel ridge regression and evolutionary algorithm [20], many studies have successfully predicted transition temperatures of liquid-crystal systems with similar methods. Neural networks or regression methods have been used to model clearing temperatures of liquid crystals (at which point a liquid crystal becomes an isotropic liquid) [21, 22], transition temperatures of bent-core liquid crystals (the upper stability limit of the mesophase) [23], nematic transition temperatures in thermotropic liquid crystals [24],

transition temperatures in binary liquid crystals [25], as well as the phase behavior of liquid crystals with a variety of classification methods (nearest-neighbor, $k$-nearest neighbor, C4.5 decision tree, random tree, random forest, reduced-error pruning tree (REPTree), nested generalized exemplar (NGE), and non-nested generalized exemplar with prototypes (NNGEP) classification) [26].

*Electronic and optical properties.* Rarer are studies of electronic and optical properties of soft materials modeled with machine learning, presumably due to the complexity of the multi-scale processes involved in these systems. A successful example is targeting bandgaps and dielectric constants in polymers modeled with a genetic algorithm [27]. Moreover, machine-learning-informed design was achieved, for example, in the discovery of electrically conducting MOFs with small bandgaps using crystal-graph convolutional neural networks [28] as well as for microstructures with maximal optical absorption performance with a generative adversarial network (GAN) [29].

*Transport Properties.* Transport properties have been modeled successfully in a variety of instances: diffusivity in porous materials with principal component analysis [30] as well as with a convolutional neural network [31]; cation diffusivity in nanoparticle-based electrolytes [32] and ionic conductivity in ceramics (yttria-stabilized zirconia), both with convolutional neural networks [33]; permeability in porous rock (Fontainebleau sandstone and Berea sandstone) [34] and seismic wave velocities in porous rock (Berea sandstone), [35], also both with convolutional neural networks. Successful design has been enabled in the case of minimal and maximal water diffusivity in hydration layers with a genetic algorithm [36] and topology optimization for heat conduction with an augmented variational autoencoder (VAE) [37].

*Chemical Properties.* Chemical properties, in particular aiming at modeling catalytic behavior, have been modeled successfully at the intersection between hard and soft matter—for example, in metal–organic framework (MOF) systems. Specific properties modeled include $CO_2$ adsorption with support vector machines [38], $CO_2$ separation–with high $CO_2$ capacity and high selectivity for $CO_2/N_2$ and $CO_2/CH_4$ separations—with a variational autoencoder [39], gas adsorption with transfer learning with deep neural networks [40], and even full adsorption isotherms of MOFs with a multilayer perceptron (MLP) [41]. Also within the realm of framework materials, binary sorption equilibria were modeled in zeolites with deep neural networks [42].

*Molecular Properties.* A variety of molecular properties have been successfully modeled for small molecules—not "soft materials", strictly speaking. Among these are:

- atomization energies for small molecules with linear ridge regression, kernel ridge regression, support vector regression, mixed-effect models, multilayer neural networks, and the $k$-nearest-neighbor method (KNN) [43];
- formation energies of small organic molecules with Gaussian process regression (GPR), combined with CUR matrix decomposition, farthest-point sampling (FPS), and a Pearson correlation (PC) method [44];
- molecular atomization energies, polarizability, and highest and lowest molecular orbital energies (HOMO and LUMO) with kernel-ridge regression (KRR) [2];

- polymorph stability and charge mobility of molecular crystals for organic electronics with Gaussian process regression [45];
- potential-energy surfaces and bond dynamics of molecules with deep tensor neural networks (DTNNs) augmented with continuous-filter convolutions with filter-generating networks [46, 47], and molecular energies, dipole moments, polarizabilities, vibrational energies, heat capacities and vibrational frequencies with Bayesian ridge regression, linear regression with elastic net regularization, random forests, kernel ridge regression, graph convolution, and gated graph networks [48];
- aqueous solubility, octanol solubility, melting point, and toxicity of small molecules with a convolutional neural network (CNN) [49];
- bioactivity of small molecules for drug discovery with deep convolutional neural networks (DCNNs) [50];
- chemical toxicity of small molecules for drug discovery with a bidirectional gated recurrent unit-based neural network (BiGRU) and a fully connected neural network (FCN) [51];
- solvation free energies, *in-vitro* HIV activity, and *in-vivo* toxicity with a deep convolutional neural network [52].

# 3 Additional reviews

We would like to point the reader to several reviews relevant to our discussion on topics that we did not expound upon in the main text. These include:

- Additional approaches for predicting polymorphic structures are discussed in a review by Price [53].
- Coarse-graining used across various domains such as polymers by Dhamankar and Webb [54], proteins by Tozzini [55], Kmiecik et al. [56], and other biomolecular systems by Noid [57], Ingólfsson et al. [58], Singh and Li [59], Liwo et al. [60].
- Polymorphism, modeling, and crystal structure prediction in pharmaceutical research by Abramov et al. [61].
- Maximizing free-energy differences between desired and undesired structures in simulation for inverse design by Torquato [62].
- Complex structures in soft matter by Dshemuchadse [63].
- Hénin et al. [64] give an overview of the different enhanced sampling methods and software implementing them.
- Sidky et al. [65] discuss ML-aided collective variable discovery for enhanced sampling instead of using ML-free descriptors described in the “Descriptors for self-assembly studies” section.
- Mehdi et al. [66] talk about the most recent developments of coupling ML-algorithms with traditional enhanced-sampling techniques.
- Soft matter roadmap by Barrat et al. [67] that includes discussion of simulation methods and inverse design.

# References


[1] Widmer-Cooper, A., Harrowell, P.: Predicting the Long-Time Dynamic Heterogeneity in a Supercooled Liquid on the Basis of Short-Time Heterogeneities. Physical Review Letters **96**(18), 185701 (2006) https://doi.org/10.1103/PhysRevLett.96.185701 . Accessed 2023-11-15

[2] Hansen, K., Biegler, F., Ramakrishnan, R., Pronobis, W., Von Lilienfeld, O.A., Müller, K.-R., Tkatchenko, A.: Machine Learning Predictions of Molecular Properties: Accurate Many-Body Potentials and Nonlocality in Chemical Space. The Journal of Physical Chemistry Letters **6**(12), 2326–2331 (2015) https://doi.org/10.1021/acs.jpclett.5b00831 . Accessed 2024-02-09

[3] Cohen, M.H., Turnbull, D.: Molecular Transport in Liquids and Glasses. The Journal of Chemical Physics **31**(5), 1164–1169 (1959) https://doi.org/10.1063/1.1730566 . Accessed 2024-03-12

[4] Barth, A.R., Martinez, M.H., Payne, C.E., Couto, C.G., Quintas, I.J., Soncharoen, I., Brown, N.M., Weissler, E.J., Gerbode, S.J.: Grain splitting is a mechanism for grain coarsening in colloidal polycrystals. Physical Review E **104**(5), 052601 (2021) https://doi.org/10.1103/PhysRevE.104.L052601 . Accessed 2024-03-12

[5] Piaggi, P.M., Parrinello, M.: Entropy based fingerprint for local crystalline order. The Journal of Chemical Physics **147**(11), 114112 (2017) https://doi.org/10.1063/1.4998408 . Accessed 2024-02-03

[6] Martiniani, S., Chaikin, P.M., Levine, D.: Quantifying Hidden Order out of Equilibrium. Physical Review X **9**(1), 011031 (2019) https://doi.org/10.1103/PhysRevX.9.011031 . Publisher: American Physical Society. Accessed 2022-12-16

[7] Sheriff, K., Cao, Y., Smidt, T., Freitas, R.: Quantifying chemical short-range order in metallic alloys. arXiv. arXiv:2311.01545 [cond-mat] (2023). https://doi.org/10.48550/arXiv.2311.01545 . http://arxiv.org/abs/2311.01545 Accessed 2024-01-05

[8] Miskin, M.Z., Jaeger, H.M.: Adapting granular materials through artificial evolution. Nature Materials **12**(4), 326–331 (2013) https://doi.org/10.1038/nmat3543 . Accessed 2024-02-01

[9] Schoenholz, S.S., Cubuk, E.D., Sussman, D.M., Kaxiras, E., Liu, A.J.: A structural approach to relaxation in glassy liquids. Nature Physics **12**(5), 469–471 (2016) https://doi.org/10.1038/nphys3644 . Accessed 2022-01-25

[10] Schoenholz, S.S., Cubuk, E.D., Kaxiras, E., Liu, A.J.: Relationship between local structure and relaxation in out-of-equilibrium glassy systems. Proceedings of the National Academy of Sciences **114**(2), 263–267 (2017) https://doi.org/10.1073/pnas.1610204114 . Accessed 2024-02-06

[11] Cubuk, E.D., Ivancic, R.J.S., Schoenholz, S.S., Strickland, D.J., Basu, A., Davidson, Z.S., Fontaine, J., Hor, J.L., Huang, Y.-R., Jiang, Y., Keim, N.C., Koshigan, K.D., Lefever, J.A., Liu, T., Ma, X.-G., Magagnosc, D.J., Morrow, E., Ortiz, C.P., Rieser, J.M., Shavit, A., Still, T., Xu, Y., Zhang, Y., Nordstrom, K.N., Arratia, P.E., Carpick, R.W., Durian, D.J., Fakhraai, Z., Jerolmack, D.J., Lee, D., Li, J., Riggleman, R., Turner, K.T., Yodh, A.G., Gianola, D.S., Liu, A.J.: Structure-property relationships from universal signatures of plasticity in disordered solids. Science **358**(6366), 1033–1037 (2017) https://doi.org/10.1126/science.aai8830 . Accessed 2024-02-06

[12] Yang, Z., Yabansu, Y.C., Al-Bahrani, R., Liao, W.-k., Choudhary, A.N., Kalidindi, S.R., Agrawal, A.: Deep learning approaches for mining structure-property linkages in high contrast composites from simulation datasets. Computational Materials Science **151**, 278–287 (2018) https://doi.org/10.1016/j.commatsci.2018.05.014 . Accessed 2024-02-06

[13] Wang, L., Chan, Y.-C., Ahmed, F., Liu, Z., Zhu, P., Chen, W.: Deep generative modeling for mechanistic-based learning and design of metamaterial systems. Computer Methods in Applied Mechanics and Engineering **372**, 113377 (2020) https://doi.org/10.1016/j.cma.2020.113377 . Accessed 2024-02-13

[14] Wang, Y., Zhang, M., Lin, A., Iyer, A., Prasad, A.S., Li, X., Zhang, Y., Schadler, L.S., Chen, W., Brinson, L.C.: Mining structure–property relationships in polymer nanocomposites using data driven finite element analysis and multi-task convolutional neural networks. Molecular Systems Design & Engineering **5**(5), 962–975 (2020) https://doi.org/10.1039/D0ME00020E . Accessed 2024-02-13

[15] Yu, C.-H., Qin, Z., Buehler, M.J.: Artificial intelligence design algorithm for nanocomposites optimized for shear crack resistance. Nano Futures **3**(3), 035001 (2019) https://doi.org/10.1088/2399-1984/ab36f0 . Accessed 2024-02-21

[16] Kumar, S., Tan, S., Zheng, L., Kochmann, D.M.: Inverse-designed spinodoid metamaterials. npj Computational Materials **6**(1), 73 (2020) https://doi.org/10.1038/s41524-020-0341-6 . Accessed 2024-02-21

[17] Kojima, T., Washio, T., Hara, S., Koishi, M.: Synthesis of computer simulation and machine learning for achieving the best material properties of filled rubber. Scientific Reports **10**(1), 18127 (2020) https://doi.org/10.1038/s41598-020-75038-0 . Accessed 2024-02-13

[18] Menon, A., Gupta, C., Perkins, K.M., DeCost, B.L., Budwal, N., Rios, R.T., Zhang, K., Póczos, B., Washburn, N.R.: Elucidating multi-physics interactions in suspensions for the design of polymeric dispersants: a hierarchical machine learning approach. Molecular Systems Design & Engineering **2**(3), 263–273 (2017) https://doi.org/10.1039/C7ME00027H . Accessed 2024-03-12

[19] Kozuch, D.J., Stillinger, F.H., Debenedetti, P.G.: Combined molecular dynamics

and neural network method for predicting protein antifreeze activity. Proceedings of the National Academy of Sciences **115**(52), 13252–13257 (2018) https://doi.org/10.1073/pnas.1814945115 . Accessed 2024-02-06

[20] Pilania, G., Iverson, C.N., Lookman, T., Marrone, B.L.: Machine-Learning-Based Predictive Modeling of Glass Transition Temperatures: A Case of Polyhydroxyalkanoate Homopolymers and Copolymers. Journal of Chemical Information and Modeling **59**(12), 5013–5025 (2019) https://doi.org/10.1021/acs.jcim.9b00807 . Accessed 2024-02-13

[21] Kränz, H., Vill, V., Meyer, B.: Prediction of Material Properties from Chemical Structures. The Clearing Temperature of Nematic Liquid Crystals Derived from Their Chemical Structures by Artificial Neural Networks. Journal of Chemical Information and Computer Sciences **36**(6), 1173–1177 (1996) https://doi.org/10.1021/ci960482r . Accessed 2024-02-21

[22] Johnson, S.R., Jurs, P.C.: Prediction of the Clearing Temperatures of a Series of Liquid Crystals from Molecular Structure. Chemistry of Materials **11**(4), 1007–1023 (1999) https://doi.org/10.1021/cm980674x . Accessed 2024-02-21

[23] Antanasijević, D., Antanasijević, J., Pocajt, V., Ušćumlić, G.: A GMDH-type neural network with multi-filter feature selection for the prediction of transition temperatures of bent-core liquid crystals. RSC Advances **6**(102), 99676–99684 (2016) https://doi.org/10.1039/C6RA15056J . Accessed 2024-02-21

[24] Xu, J., Wang, L., Zhang, H., Yi, C., Xu, W.: Accurate quantitative structure–property relationship analysis for prediction of nematic transition temperatures in thermotropic liquid crystals. Molecular Simulation **36**(1), 26–34 (2010) https://doi.org/10.1080/08927020903096064 . Accessed 2024-02-21

[25] Inokuchi, T., Okamoto, R., Arai, N.: Predicting molecular ordering in a binary liquid crystal using machine learning. Liquid Crystals **47**(3), 438–448 (2020) https://doi.org/10.1080/02678292.2019.1656293 . Accessed 2024-02-21

[26] Leon, F., Lisa, C., Curteanu, S.: Prediction of the Liquid-Crystalline Property Using Different Classification Methods. Molecular Crystals and Liquid Crystals **518**(1), 129–148 (2010) https://doi.org/10.1080/15421400903574391 . Accessed 2024-02-21

[27] Mannodi-Kanakkithodi, A., Pilania, G., Huan, T.D., Lookman, T., Ramprasad, R.: Machine Learning Strategy for Accelerated Design of Polymer Dielectrics. Scientific Reports **6**(1), 20952 (2016) https://doi.org/10.1038/srep20952 . Accessed 2024-02-13

[28] Rosen, A.S., Iyer, S.M., Ray, D., Yao, Z., Aspuru-Guzik, A., Gagliardi, L., Notestein, J.M., Snurr, R.Q.: Machine learning the quantum-chemical properties of metal–organic frameworks for accelerated materials discovery. Matter

4(5), 1578–1597 (2021) https://doi.org/10.1016/j.matt.2021.02.015 . Accessed 2024-02-13

[29] Yang, Z., Li, X., Catherine Brinson, L., Choudhary, A.N., Chen, W., Agrawal, A.: Microstructural Materials Design Via Deep Adversarial Learning Methodology. Journal of Mechanical Design **140**(11), 111416 (2018) https://doi.org/10.1115/1.4041371 . Accessed 2024-02-06

[30] Çeçen, A., Fast, T., Kumbur, E.C., Kalidindi, S.R.: A data-driven approach to establishing microstructure–property relationships in porous transport layers of polymer electrolyte fuel cells. Journal of Power Sources **245**, 144–153 (2014) https://doi.org/10.1016/j.jpowsour.2013.06.100 . Accessed 2024-02-06

[31] Wu, H., Fang, W.-Z., Kang, Q., Tao, W.-Q., Qiao, R.: Predicting Effective Diffusivity of Porous Media from Images by Deep Learning. Scientific Reports **9**(1), 20387 (2019) https://doi.org/10.1038/s41598-019-56309-x . Accessed 2024-02-20

[32] Kadulkar, S., Howard, M.P., Truskett, T.M., Ganesan, V.: Prediction and Optimization of Ion Transport Characteristics in Nanoparticle-Based Electrolytes Using Convolutional Neural Networks. The Journal of Physical Chemistry B **125**(18), 4838–4849 (2021) https://doi.org/10.1021/acs.jpcb.1c02004 . Accessed 2024-02-13

[33] Kondo, R., Yamakawa, S., Masuoka, Y., Tajima, S., Asahi, R.: Microstructure recognition using convolutional neural networks for prediction of ionic conductivity in ceramics. Acta Materialia **141**, 29–38 (2017) https://doi.org/10.1016/j.actamat.2017.09.004 . Accessed 2024-02-20

[34] Srisutthiyakorn*, N.: Deep-learning methods for predicting permeability from 2D/3D binary-segmented images. In: SEG Technical Program Expanded Abstracts 2016, pp. 3042–3046. Society of Exploration Geophysicists, Dallas, Texas (2016). https://doi.org/10.1190/segam2016-13972613.1 . https://library.seg.org/doi/10.1190/segam2016-13972613.1 Accessed 2024-02-20

[35] Karimpouli, S., Tahmasebi, P.: Image-based velocity estimation of rock using Convolutional Neural Networks. Neural Networks **111**, 89–97 (2019) https://doi.org/10.1016/j.neunet.2018.12.006 . Accessed 2024-02-20

[36] Monroe, J.I., Shell, M.S.: Computational discovery of chemically patterned surfaces that effect unique hydration water dynamics. Proceedings of the National Academy of Sciences **115**(32), 8093–8098 (2018) https://doi.org/10.1073/pnas.1807208115 . Accessed 2024-02-01

[37] Guo, T., Lohan, D.J., Cang, R., Ren, M.Y., Allison, J.T.: An Indirect Design Representation for Topology Optimization Using Variational Autoencoder and Style Transfer. In: 2018 AIAA/ASCE/AHS/ASC Structures, Structural Dynamics,

and Materials Conference. American Institute of Aeronautics and Astronautics, Kissimmee, Florida (2018). https://doi.org/10.2514/6.2018-0804 . https://arc.aiaa.org/doi/10.2514/6.2018-0804 Accessed 2024-02-06

[38] Fernandez, M., Boyd, P.G., Daff, T.D., Aghaji, M.Z., Woo, T.K.: Rapid and Accurate Machine Learning Recognition of High Performing Metal Organic Frameworks for $CO_2$ Capture. The Journal of Physical Chemistry Letters **5**(17), 3056–3060 (2014) https://doi.org/10.1021/jz501331m . Accessed 2024-03-13

[39] Yao, Z., Sánchez-Lengeling, B., Bobbitt, N.S., Bucior, B.J., Kumar, S.G.H., Collins, S.P., Burns, T., Woo, T.K., Farha, O.K., Snurr, R.Q., Aspuru-Guzik, A.: Inverse design of nanoporous crystalline reticular materials with deep generative models. Nature Machine Intelligence **3**(1), 76–86 (2021) https://doi.org/10.1038/s42256-020-00271-1 . Accessed 2024-02-13

[40] Ma, R., Colón, Y.J., Luo, T.: Transfer Learning Study of Gas Adsorption in Metal–Organic Frameworks. ACS Applied Materials & Interfaces **12**(30), 34041–34048 (2020) https://doi.org/10.1021/acsami.0c06858 . Accessed 2024-03-13

[41] Anderson, R., Biong, A., Gómez-Gualdrón, D.A.: Adsorption Isotherm Predictions for Multiple Molecules in MOFs Using the Same Deep Learning Model. Journal of Chemical Theory and Computation **16**(2), 1271–1283 (2020) https://doi.org/10.1021/acs.jctc.9b00940 . Accessed 2024-03-13

[42] Sun, Y., DeJaco, R.F., Siepmann, J.I.: Deep neural network learning of complex binary sorption equilibria from molecular simulation data. Chemical Science **10**(16), 4377–4388 (2019) https://doi.org/10.1039/C8SC05340E . Accessed 2024-03-13

[43] Hansen, K., Montavon, G., Biegler, F., Fazli, S., Rupp, M., Scheffler, M., Von Lilienfeld, O.A., Tkatchenko, A., Müller, K.-R.: Assessment and Validation of Machine Learning Methods for Predicting Molecular Atomization Energies. Journal of Chemical Theory and Computation **9**(8), 3404–3419 (2013) https://doi.org/10.1021/ct400195d . Accessed 2024-02-09

[44] Imbalzano, G., Anelli, A., Giofré, D., Klees, S., Behler, J., Ceriotti, M.: Automatic selection of atomic fingerprints and reference configurations for machine-learning potentials. The Journal of Chemical Physics **148**(24), 241730 (2018) https://doi.org/10.1063/1.5024611 . Accessed 2024-02-09

[45] Musil, F., De, S., Yang, J., Campbell, J.E., Day, G.M., Ceriotti, M.: Machine learning for the structure–energy–property landscapes of molecular crystals. Chemical Science **9**(5), 1289–1300 (2018) https://doi.org/10.1039/C7SC04665K . Accessed 2024-02-12

[46] Schütt, K.T., Arbabzadah, F., Chmiela, S., Müller, K.R., Tkatchenko, A.:

Quantum-chemical insights from deep tensor neural networks. Nature Communications **8**(1), 13890 (2017) https://doi.org/10.1038/ncomms13890 . Accessed 2024-02-12

[47] Schütt, K.T., Sauceda, H.E., Kindermans, P.-J., Tkatchenko, A., Müller, K.-R.: SchNet – A deep learning architecture for molecules and materials. The Journal of Chemical Physics **148**(24), 241722 (2018) https://doi.org/10.1063/1.5019779 . Accessed 2024-02-12

[48] Faber, F.A., Hutchison, L., Huang, B., Gilmer, J., Schoenholz, S.S., Dahl, G.E., Vinyals, O., Kearnes, S., Riley, P.F., Von Lilienfeld, O.A.: Prediction Errors of Molecular Machine Learning Models Lower than Hybrid DFT Error. Journal of Chemical Theory and Computation **13**(11), 5255–5264 (2017) https://doi.org/10.1021/acs.jctc.7b00577 . Accessed 2024-02-12

[49] Coley, C.W., Barzilay, R., Green, W.H., Jaakkola, T.S., Jensen, K.F.: Convolutional Embedding of Attributed Molecular Graphs for Physical Property Prediction. Journal of Chemical Information and Modeling **57**(8), 1757–1772 (2017) https://doi.org/10.1021/acs.jcim.6b00601 . Accessed 2024-02-19

[50] Wallach, I., Dzamba, M., Heifets, A.: AtomNet: A Deep Convolutional Neural Network for Bioactivity Prediction in Structure-based Drug Discovery (2015) https://doi.org/10.48550/ARXIV.1510.02855 . Publisher: arXiv Version Number: 1. Accessed 2024-02-19

[51] Peng, Y., Zhang, Z., Jiang, Q., Guan, J., Zhou, S.: TOP: Towards Better Toxicity Prediction by Deep Molecular Representation Learning. In: 2019 IEEE International Conference on Bioinformatics and Biomedicine (BIBM), pp. 318–325. IEEE, San Diego, CA, USA (2019). https://doi.org/10.1109/BIBM47256.2019.8983340 . https://ieeexplore.ieee.org/document/8983340/ Accessed 2024-02-19

[52] Goh, G.B., Siegel, C., Vishnu, A., Hodas, N.O., Baker, N.: Chemception: A Deep Neural Network with Minimal Chemistry Knowledge Matches the Performance of Expert-developed QSAR/QSPR Models (2017) https://doi.org/10.48550/ARXIV.1706.06689 . Publisher: arXiv Version Number: 1. Accessed 2024-02-20

[53] Price, S.L.: From crystal structure prediction to polymorph prediction: interpreting the crystal energy landscape. Physical Chemistry Chemical Physics **10**(15), 1996–2009 (2008) https://doi.org/10.1039/B719351C . Publisher: The Royal Society of Chemistry. Accessed 2024-03-08

[54] Dhamankar, S., Webb, M.A.: Chemically specific coarse-graining of polymers: Methods and prospects. Journal of Polymer Science **59**(22), 2613–2643 (2021) https://doi.org/10.1002/pol.20210555 . _eprint: https://onlinelibrary.wiley.com/doi/pdf/10.1002/pol.20210555. Accessed 2024-02-27

[55] Tozzini, V.: Coarse-grained models for proteins. Current Opinion in Structural Biology **15**(2), 144–150 (2005) https://doi.org/10.1016/j.sbi.2005.02.005 . Accessed 2024-02-27

[56] Kmiecik, S., Gront, D., Kolinski, M., Wieteska, L., Dawid, A.E., Kolinski, A.: Coarse-Grained Protein Models and Their Applications. Chemical Reviews **116**(14), 7898–7936 (2016) https://doi.org/10.1021/acs.chemrev.6b00163 . Publisher: American Chemical Society. Accessed 2024-02-27

[57] Noid, W.G.: Perspective: Coarse-grained models for biomolecular systems. The Journal of Chemical Physics **139**(9), 090901 (2013) https://doi.org/10.1063/1.4818908 . Accessed 2024-02-23

[58] Ingólfsson, H.I., Lopez, C.A., Uusitalo, J.J., Jong, D.H., Gopal, S.M., Periole, X., Marrink, S.J.: The power of coarse graining in biomolecular simulations. Wiley Interdisciplinary Reviews. Computational Molecular Science **4**(3), 225–248 (2014) https://doi.org/10.1002/wcms.1169 . Accessed 2024-02-27

[59] Singh, N., Li, W.: Recent Advances in Coarse-Grained Models for Biomolecules and Their Applications. International Journal of Molecular Sciences **20**(15), 3774 (2019) https://doi.org/10.3390/ijms20153774 . Accessed 2024-02-27

[60] Liwo, A., Czaplewski, C., Sieradzan, A.K., Lipska, A.G., Samsonov, S.A., Murarka, R.K.: Theory and Practice of Coarse-Grained Molecular Dynamics of Biologically Important Systems. Biomolecules **11**(9), 1347 (2021) https://doi.org/10.3390/biom11091347 . Number: 9 Publisher: Multidisciplinary Digital Publishing Institute. Accessed 2024-02-27

[61] Abramov, Y.A., Sun, G., Zeng, Q.: Emerging Landscape of Computational Modeling in Pharmaceutical Development. Journal of Chemical Information and Modeling **62**(5), 1160–1171 (2022) https://doi.org/10.1021/acs.jcim.1c01580 . Publisher: American Chemical Society. Accessed 2024-02-27

[62] Torquato, S.: Inverse optimization techniques for targeted self-assembly. Soft Matter **5**(6), 1157–1173 (2009) https://doi.org/10.1039/B814211B . Publisher: The Royal Society of Chemistry. Accessed 2024-03-10

[63] Dshemuchadse, J.: Soft matter crystallography—Complex, diverse, and new crystal structures in condensed materials on the mesoscale. Journal of Applied Physics **131**(2), 020901 (2022) https://doi.org/10.1063/5.0072017 . Publisher: American Institute of Physics. Accessed 2023-02-21

[64] Hénin, J., Lelièvre, T., Shirts, M.R., Valsson, O., Delemotte, L.: Enhanced Sampling Methods for Molecular Dynamics Simulations [Article v1.0]. Living Journal of Computational Molecular Science **4**(1), 1583–1583 (2022) https://doi.org/10.33011/livecoms.4.1.1583 . Number: 1. Accessed 2024-03-13

[65] Sidky, H., Chen, W., Ferguson, A.L.: Machine learning for collective variable discovery and enhanced sampling in biomolecular simulation. Molecular Physics **118**(5), 1737742 (2020) https://doi.org/10.1080/00268976.2020.1737742 . Publisher: Taylor & Francis _eprint: https://doi.org/10.1080/00268976.2020.1737742. Accessed 2024-01-04

[66] Mehdi, S., Smith, Z., Herron, L., Zou, Z., Tiwary, P.: Enhanced Sampling with Machine Learning. Annual Review of Physical Chemistry **75**(1), (2024) https://doi.org/10.1146/annurev-physchem-083122-125941 . _eprint: https://doi.org/10.1146/annurev-physchem-083122-125941. Accessed 2024-03-12

[67] Barrat, J.-L., Del Gado, E., Egelhaaf, S.U., Mao, X., Dijkstra, M., Pine, D.J., Kumar, S.K., Bishop, K., Gang, O., Obermeyer, A., Papadakis, C.M., Tsitsilianis, C., Smalyukh, I.I., Hourlier-Fargette, A., Andrieux, S., Drenckhan, W., Wagner, N., Murphy, R.P., Weeks, E.R., Cerbino, R., Han, Y., Cipelletti, L., Ramos, L., Poon, W.C.K., Richards, J.A., Cohen, I., Furst, E.M., Nelson, A., Craig, S.L., Ganapathy, R., Sood, A.K., Sciortino, F., Mungan, M., Sastry, S., Scheibner, C., Fruchart, M., Vitelli, V., Ridout, S.A., Stern, M., Tah, I., Zhang, G., Liu, A.J., Osuji, C.O., Xu, Y., Shewan, H.M., Stokes, J.R., Merkel, M., Ronceray, P., Rupprecht, J.-F., Matsarskaia, O., Schreiber, F., Roosen-Runge, F., Aubin-Tam, M.-E., Koenderink, G.H., Espinosa-Marzal, R.M., Yus, J., Kwon, J.: Soft matter roadmap *. Journal of Physics: Materials **7**(1), 012501 (2024) https://doi.org/10.1088/2515-7639/ad06cc . Accessed 2024-01-19
